# Supplementary material for: The Effects of Political Martyrdom on Election Results: The Assassination of Abe
Source: arXiv:2305.18004 source file (2023-08-28)
Supplement: Supplementary file 1 [file appendix.tex]

\begin{figure*}
        \centering
        \includegraphics[width=\textwidth]{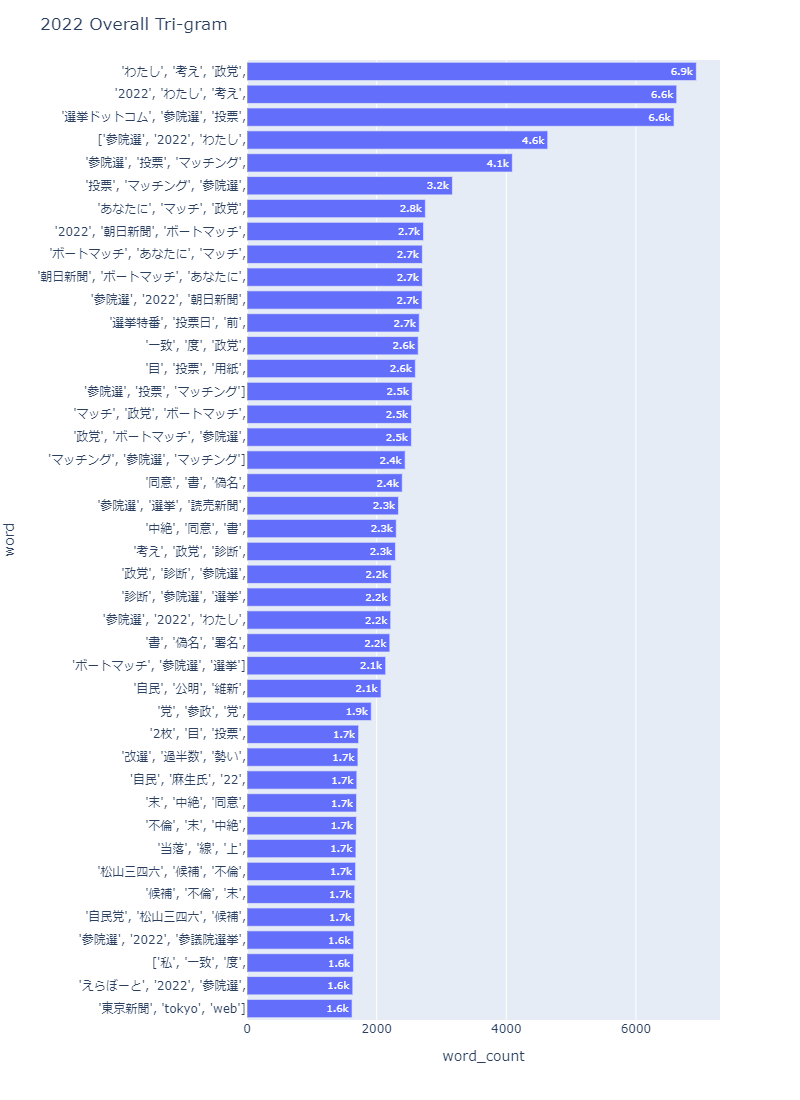}
        \caption{Trigram for Overall 2022 Election Period}
        \label{fig:2022 Overall Trigram}
\end{figure*}

\begin{figure*}
        \centering
        \includegraphics[width=\textwidth]{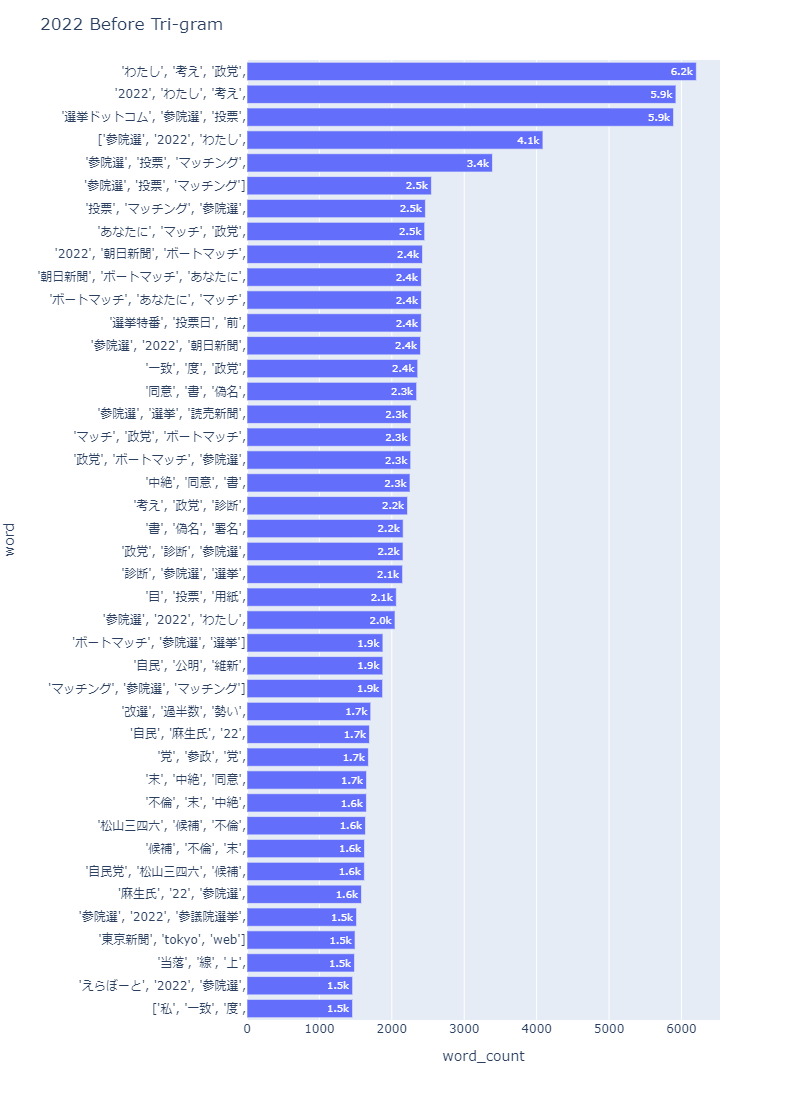}
        \caption{Trigram for Period Before Assassination}
        \label{fig:Before Assassination}
\end{figure*}

\begin{figure*}
        \centering
        \includegraphics[width=\textwidth]{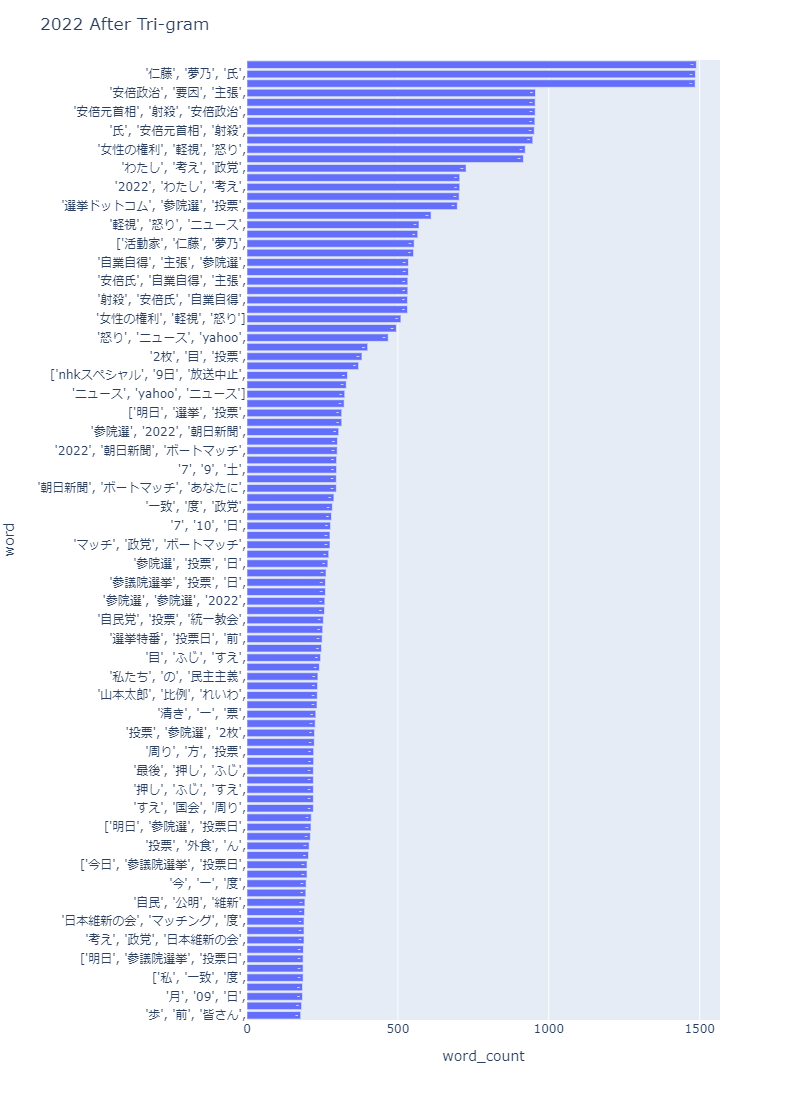}
        \caption{Trigram for Period After Assassination}
        \label{fig:After Assassination}
\end{figure*}
